# Supplementary material for: Jupybara: Operationalizing a Design Space for Actionable Data Analysis and Storytelling with LLMs
Source: arXiv:2501.16661 source file (2025-01-28)
Supplement: Supplementary file 1 [file 10-appendix.tex]

\begin{figure*}[t]
  \centering
  \includegraphics[width=\textwidth]{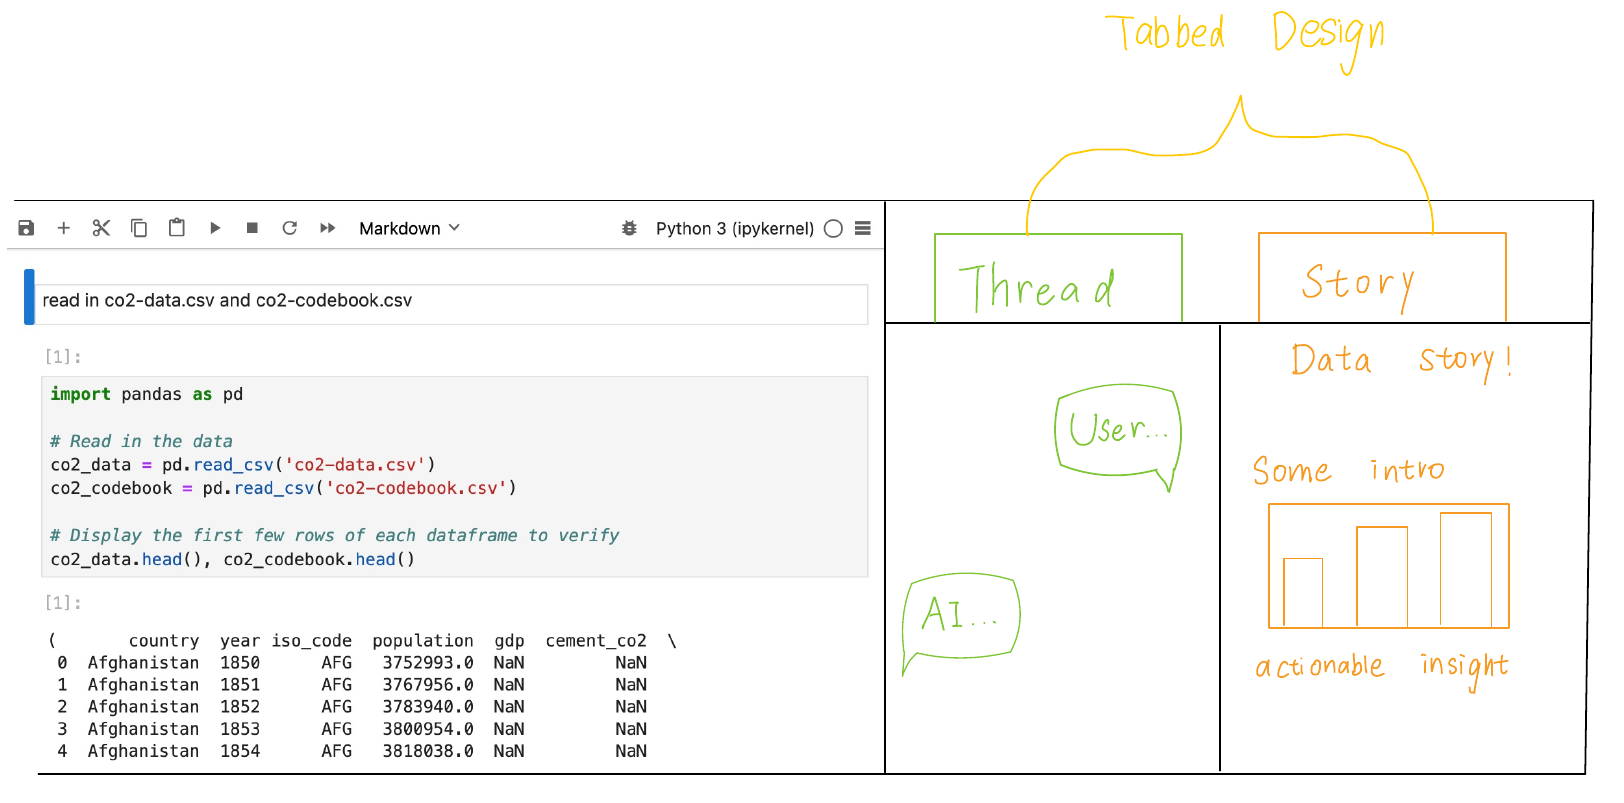}
  \caption{Screenshot of the interface design of the Jupyter Notebook extension proposed by a participant in one of the co-design sessions, which inspired our adoption of a side panel for data storytelling in the final design.}
  \label{fig:codesign}
\end{figure*}
