# Supplementary material for: Jupybara: Operationalizing a Design Space for Actionable Data Analysis and Storytelling with LLMs
Source: arXiv:2501.16661 source file (2025-01-28)
Supplement: Supplementary file 2 [file supplementary.tex]

\begin{figure*}[t]
    \centering 
    \includegraphics[width=\textwidth]{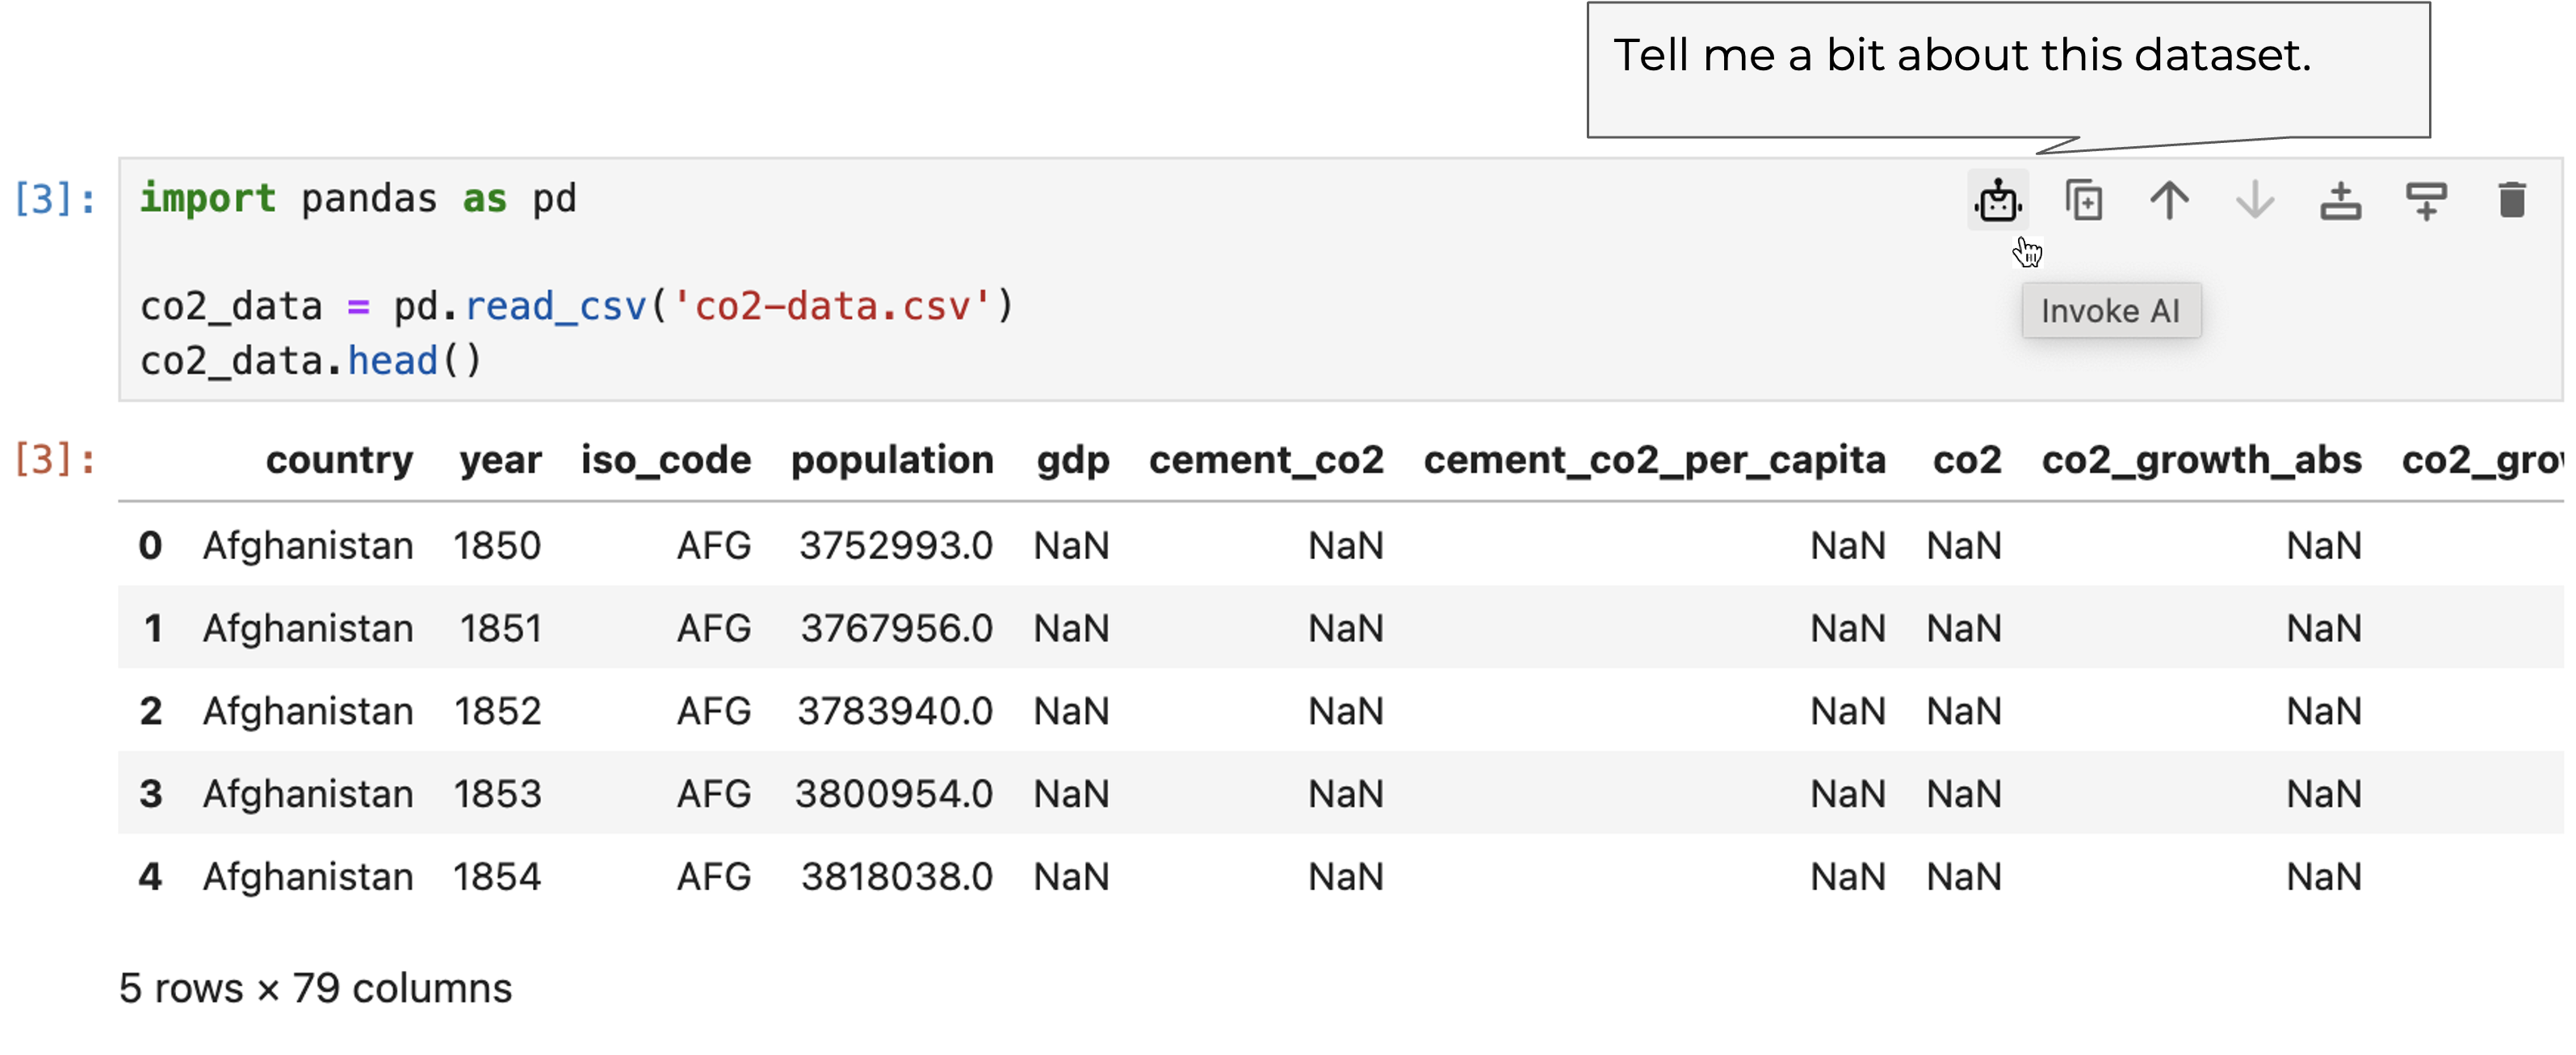}
    \caption{The \textcolor{teal}{targeted cell} design exposes an input area for user queries via a popover  specific to each cell. The popover is activated upon clicking the "Invoke AI" button on the cell toolbar.}
    \label{fig:targeted cell}
\end{figure*}

\begin{figure*}[t]
    \centering 
    \includegraphics[width=\textwidth]{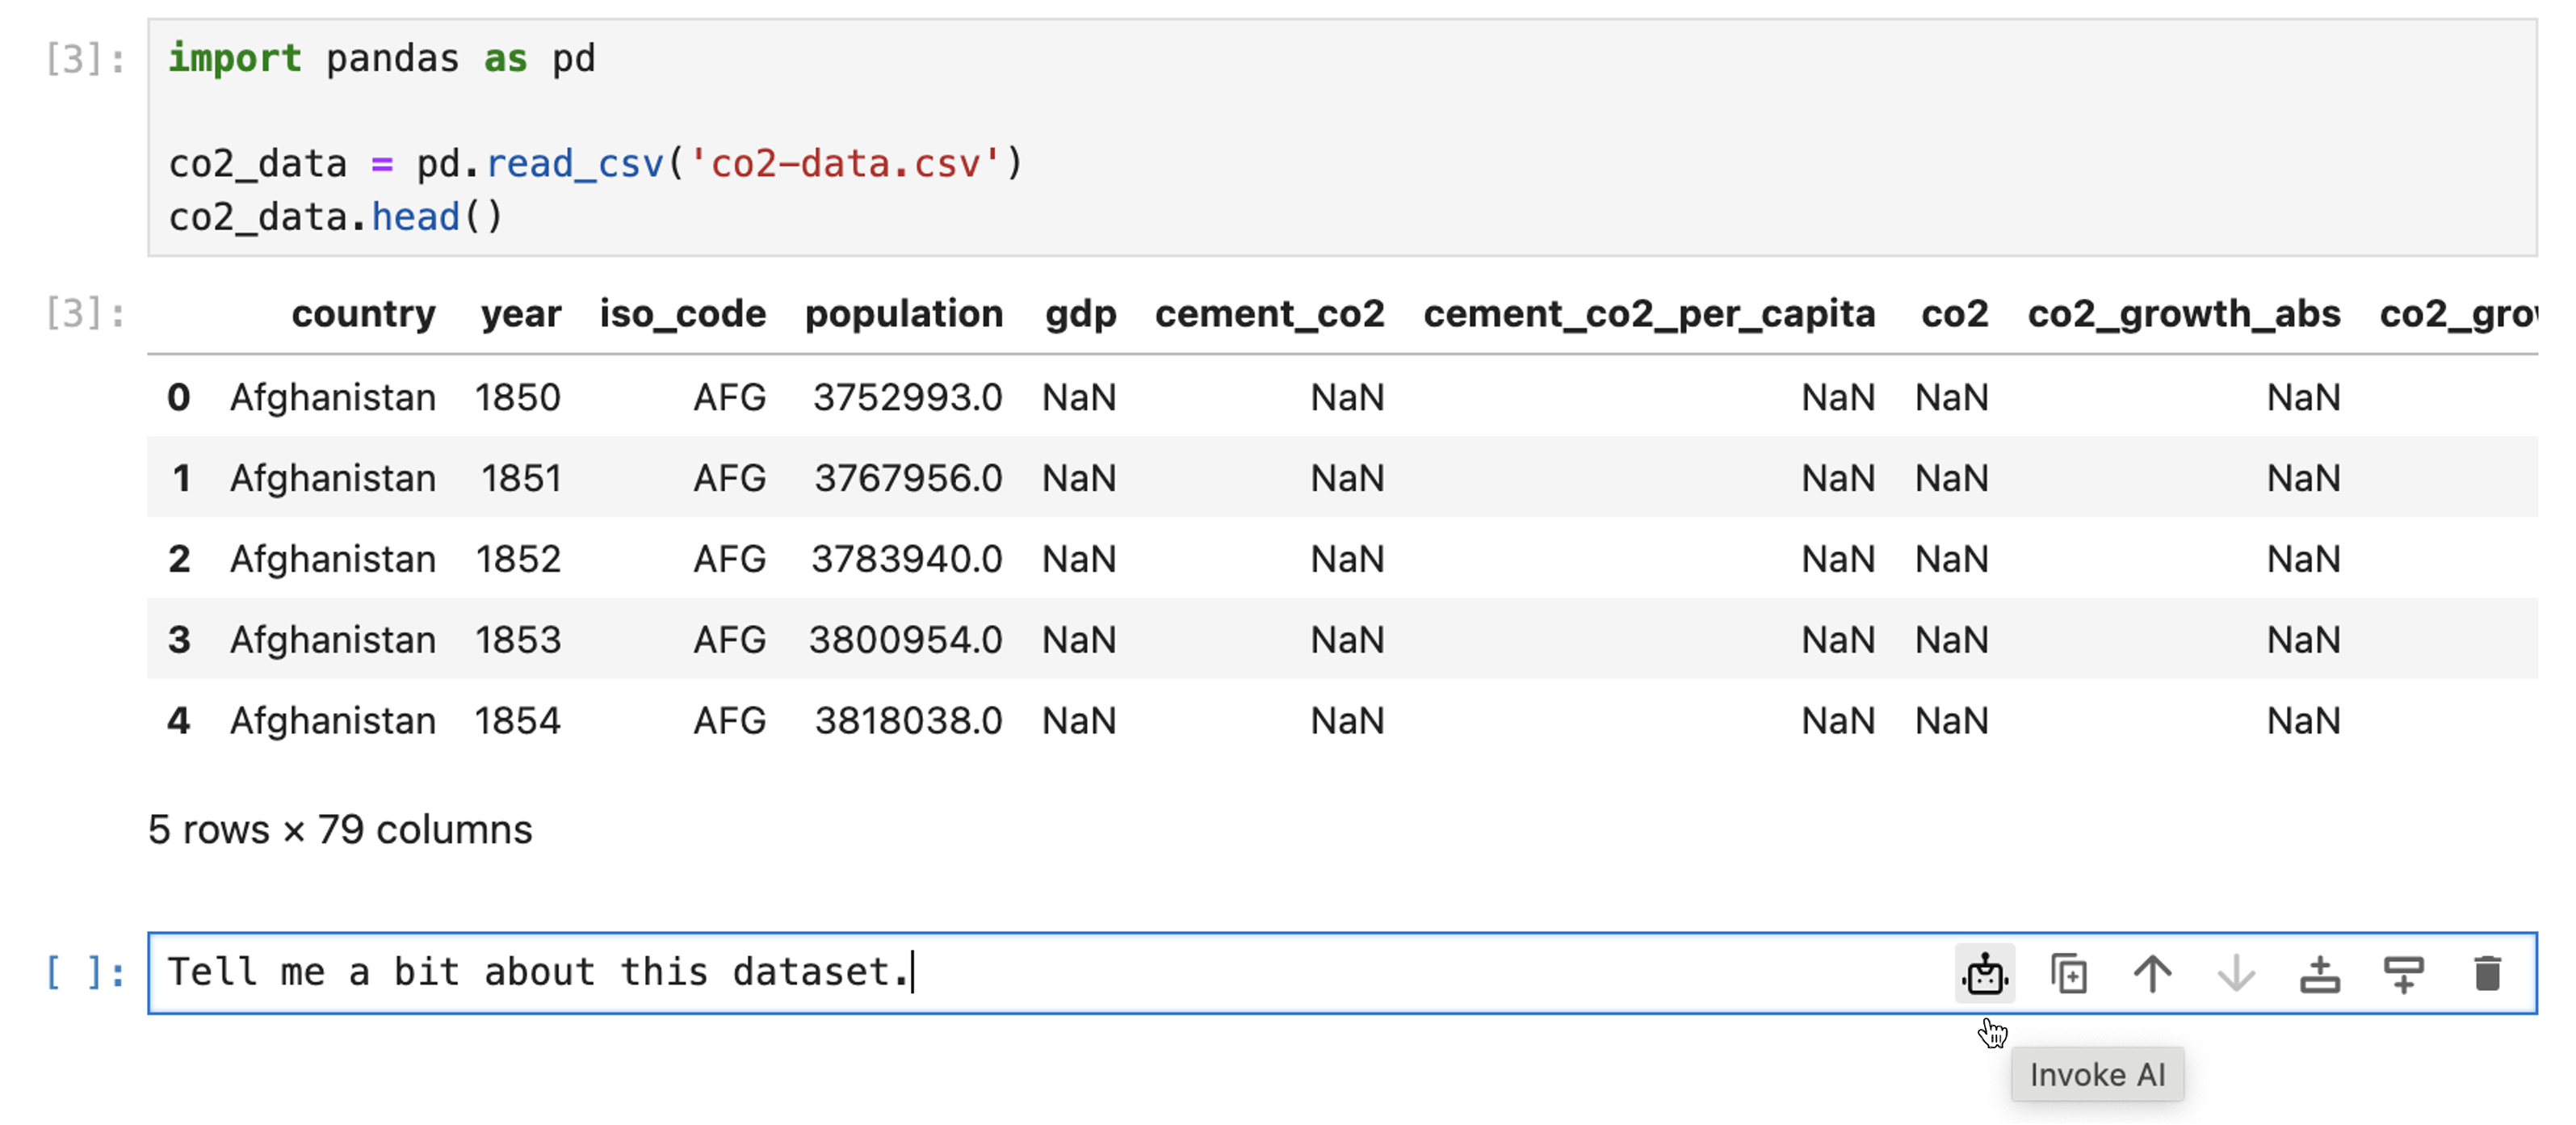}
    \caption{The \textcolor{lightpink}{inline cell} design places input areas in separate cells between normal notebook cells. Users can send queries to the AI assistant by clicking the "Invoke AI" button on the cell toolbar.}
    \label{fig:inline}
\end{figure*}

\begin{figure*}[t]
    \centering 
    \includegraphics[width=\textwidth]{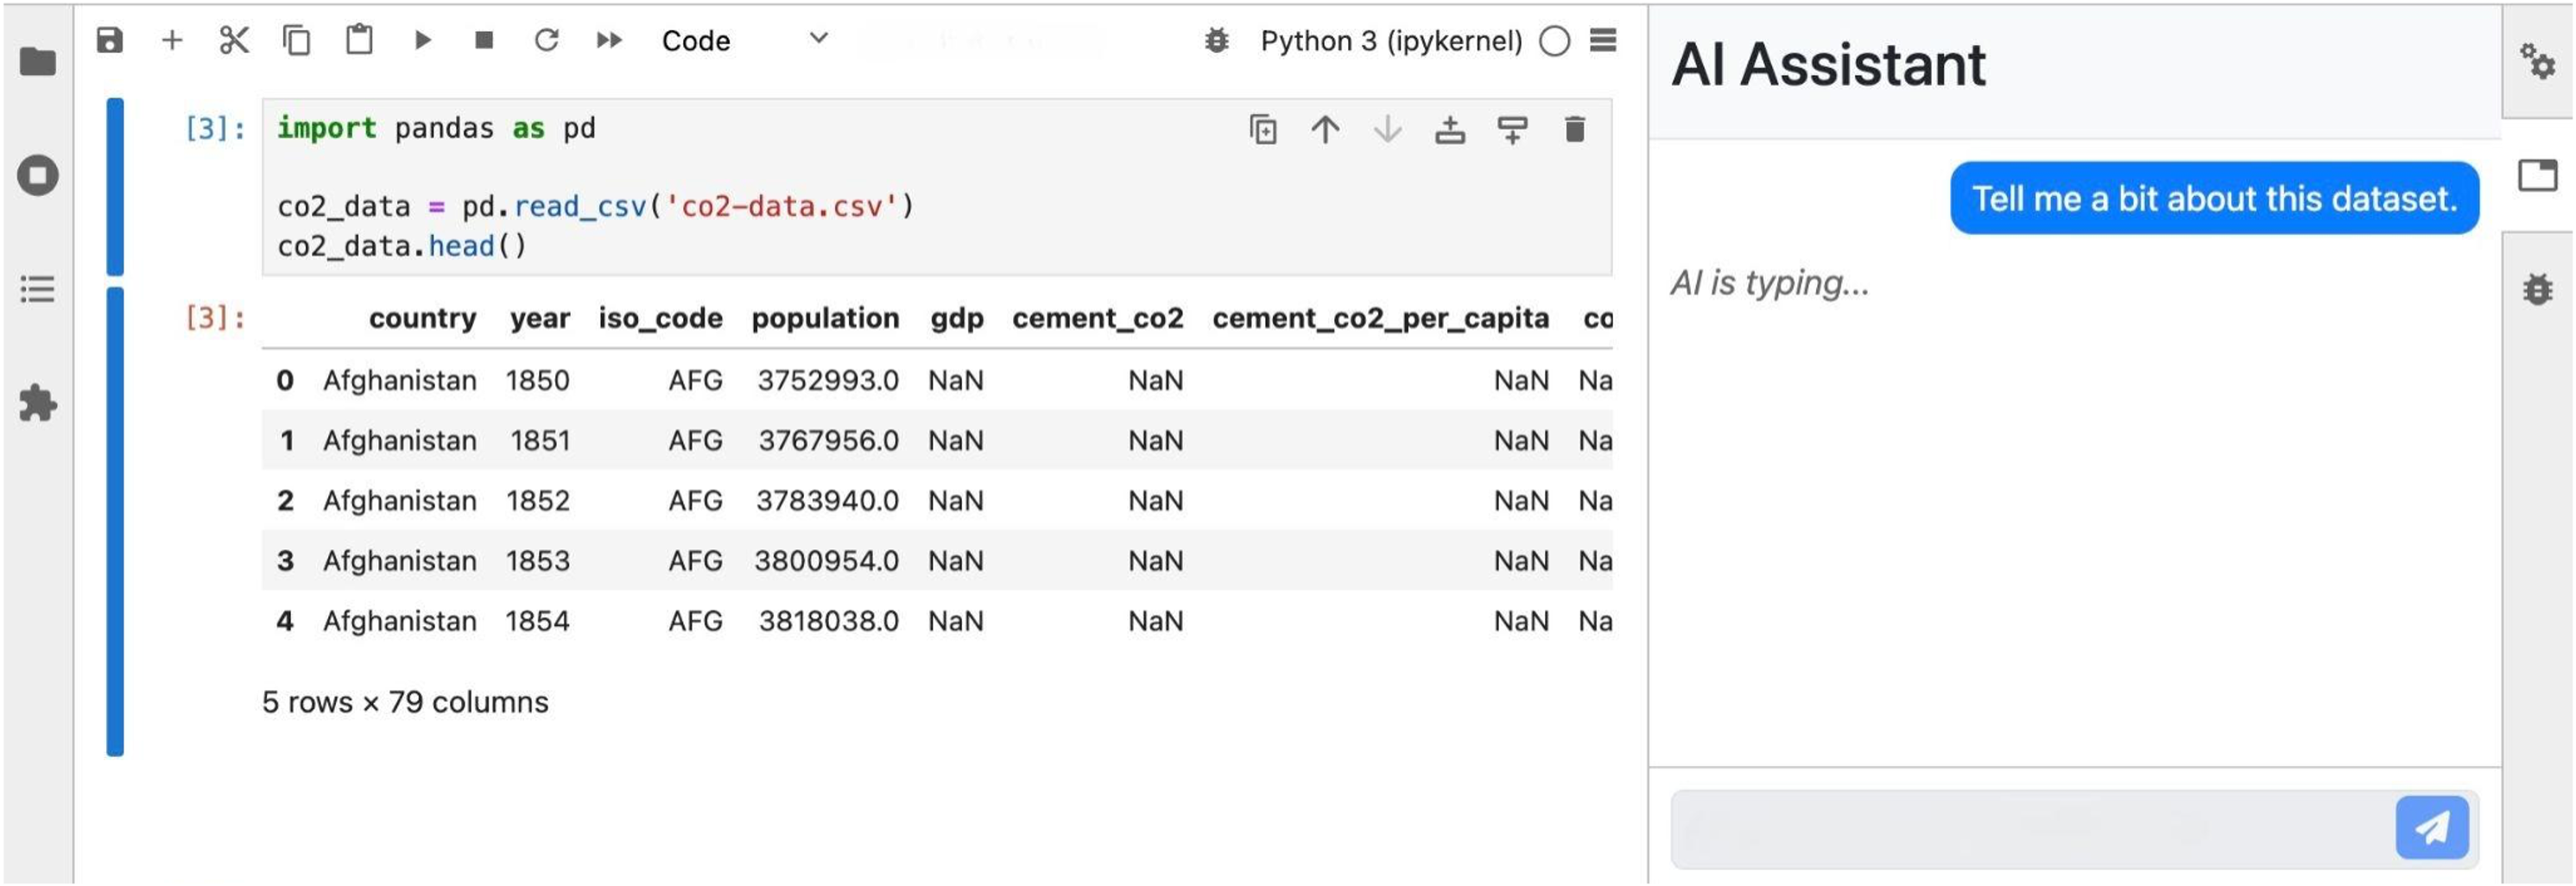}
    \caption{The \textcolor{lightblue}{side panel} design adds a separate interface by the side of the main working area of the notebook. Users can input queries in a message box.}
    \label{fig:side panel}
\end{figure*}
